# Supplementary material for: Domain Adaptation and Entanglement: an Optimal Transport Perspective
Source: arXiv:2503.08155 source file (2025-03-11)
Supplement: Supplementary file 1 [file removed.tex]

\paragraph{Remark.} The term $W_{1,l}(f \# p, f \# \hat{p}, p)$ in Theorem~\ref{thm:gen-finite-Y} suggests a new regularization scheme using optimal transport: in each mini-batch (that is sufficiently large), we can separate the mini-batch of size $2N$ into two mini-batches of size $N$ (in a class-balanced way) and apply optimal transport between them. The cost of the optimal transport is to be added to the empirical risk at each step.\\

\paragraph{Remark.} The typical optimal transport bounds, see e.g. \cite{bolley2007, boucheron2013concentration} depend on the dimension $M$ of the (in our case output) space in a prohibitive way, e.g. for a neural network with $10$ classes as output, if we would like the empirical Wasserstein distance to be close to the actual distance within $\epsilon = 0.01$ with high probability greater than $1 - \delta, \delta = 0.1$, then we'd need roughly $N, N' \sim 10^{20}$ samples! 
%However standard ML datasets containing e.g. natural images show much faster concentration and hence we conjecture that the $d$-dependency can be replaced with an appropriate complexity measure such as the VC-dimension. Intuitively this is because samples from $p, q$ are only accessed in the optimal transport through the embedding $f$.

\section{Assumptions Removed}

\fix{Alex: Good place for this? Maybe appending with a remark to replace it.}
\begin{corollary} \label{cor:partial-marginal-lipschitz}
    Let $c \colon (\mathcal{X} \times \mathcal{Y}) \times (\mathcal{X} \times
    \mathcal{Y}) \rightarrow \mathbb{R}$ be a decomposable cost function that
    decomposes into cost functions $c_1 \colon \mathcal{X} \times \mathcal{X}
    \rightarrow \mathbb{R}$ and $c_2 \colon \mathcal{Y} \times \mathcal{Y}
    \rightarrow \mathbb{R}$.
    Furthermore, let $1 \leq p < \infty$. 
    
    If $\vert c_{1} \vert \leq L $ then,
    \begin{align}
        W_{p, c}(\mu, \nu) &\leq L \cdot \TV^{1/p}(\mu_{\rm x}, \nu_{\rm x}) + \expect_{(x, x') \sim \gamma_{x}^{\star}}\left[W_{p, c_2}^{p}(\mu_{\rm y \mid x}(\cdot \mid x), \nu_{\rm y \mid x}(\cdot \mid x')) \right]^{1/p},
    \end{align}
    where $\gamma_x^{\TV}$ is the optimal couplings corresponding to total variation $\TV(\mu_{\rm x}, \nu_{\rm x})$.

    Similarly, if $\vert c_{2} \vert \leq L $ then,
    \begin{align}
        W_{p, c}(\mu, \nu) &\leq L \cdot \TV^{1/p}(\mu_{\rm y}, \nu_{\rm y}) + \expect_{(y, y') \sim \gamma_{y}^{\star}}\left[W_{p, c_1}^{p}(\mu_{\rm x \mid y}(\cdot \mid y), \nu_{\rm x \mid y}(\cdot \mid y')) \right]^{1/p},
    \end{align}
    where $\gamma_y^{\TV}$ is the optimal couplings corresponding to total variation $\TV(\mu_{\rm y}, \nu_{\rm y})$.
\end{corollary}
\begin{proof}[Proof Sketch]
    The proof is identical to Lemma~\ref{lemma2} with an additional upper bound on the appropriate cost function ($c_1$ or $c_2$) with $L$ times the Kronecker cost function.
\end{proof}

\subsection{Concentration inequalities} % and application to standard generalization

The bound in Lemma~\ref{lemma1} is also useful in the standard \iid setting where the target distribution is the original source distribution and we only have $N$ samples from it (i.e. the source is the empirical distribution $\hat{p}(x,y)$ and target is $p(x,y)$). A simple generalization bound can be obtained by exploiting concentration properties of Wasserstein distances.
\begin{theorem}\label{thm:gen-finite-Y}
    Let $\hat{p} \in \triangle(\mathcal{X} \times \mathcal{Y})$ be a empirical probability measure of $p \in \triangle(\mathcal{X} \times \mathcal{Y})$ generated by $N$ samples in the classification setting, \ie, $\vert \mathcal{Y} \vert < \infty$. Suppose that the loss function $\ell \colon \mathcal{Y} \times \mathcal{Y} \rightarrow \mathbb{R}$ satisfies metric properties and is also bounded such that $ \vert \ell \vert \leq L $. Then for any surjective model $f \colon \mathcal{X} \rightarrow \mathcal{Y}$, 
    \begin{equation}
        \risk_{p}(f) 
        \leq \emprisk_{p}(f) + W_{1, \ell, \ell}(f\#p, f\#\hat{p})
        \leq \emprisk_{p}(f) + 
        L \cdot \vert \mathcal{Y} \vert^2 \cdot \sqrt{\frac{1}{2N} \cdot \log \left( \frac{2 \vert \mathcal{Y} \vert^2}{\delta} \right)},
    \end{equation}
    holds with at least $1-\delta$ probability.
\end{theorem}

\fix{TODO: Typically Bolley et al., 2007 is used for DA. Make a note for other papers (JDOT, DA OT Gen). }

\fix{TODO: delete 4.1? Reevaluate the importance of lemma 4.1 or 4.2 by re-reading the section.}

\fix{Alex: There is a variant where you can potentially (?) account for small distances on the conditionals ... I am going to write it for Lem 4.3. Basic sketch is to reduce the marginal Wasserstein to be that \wrt the discrete metric. Then we know exactly the optimal coupling is equal to.}

\fix{Alex: I was thinking if ordering of diagonal elements sums are a result of OT plans. But I don't think this works. With a very lopsided cost, I don't see why it should particularly hold. }

\begin{lemma}\label{lemma41}
  Whenever the CCA($\alpha$) holds for some $\alpha \geq 0$ and the Wasserstein-1 distance between the label distributions $W_{1, \ell}(p_y, q_y) \leq \delta$ for some small $\delta > 0$, then CDA assumption also holds with $\lambda := 2 \alpha + \tfrac{B+m}{m}\delta$ where $B$ is a upper bound on the loss and $m$ is a lower bound on the loss evaluated on different labels: $m := \min_{y \neq y'}\ell(y, y')$.
\end{lemma}

\begin{proof}
For notational convenience we refer to the diagonal and nondiagonal elements of the matrix $W_{1,l}(f^{*} \#p_{x \mid y}(\cdot \mid y), f^{*} \#q_{x \mid y}(\cdot \mid y')$ as $W_{yy}(f^*)$ and $W_{y,y'}(f^*)$ below. Using the second upper bound in Lemma~\ref{lemma2} for 1-Wasserstein distances
\begin{align*}
  \risk_q(f^{*}) &\leq \risk_p(f^{*}) + \sum_{y, y'} \gamma_{y}^{\star}(y, y') W_{1,l}(f^* \# p_{x \mid y}(\cdot \mid y), f^{*} \# q_{x \mid y}(\cdot \mid y')) + \delta \\
  &\leq \risk_p(f^{*}) + \max_y W_{yy}(f^*) + \sum_{y \neq y'}\gamma_{y}^{\star}(y,y')W_{yy'}(f^*) + \delta \\
  &\leq \alpha + B\sum_{y \neq y'}\gamma_y^*(y,y') + \delta
\end{align*}
where $f^{*}$ is the classifier minimizing the right hand side. In the second and inequalities we separated the diagonal and nondiagonal entries of the $M \times M$ matrix $\gamma_y^{\star}(y, y')$ and bounded each separately. Next we use the fact that $W_{1, \ell}(p_y, q_y) \leq \delta$ for some small $\delta >0$ implies that $\gamma_y^*(y,y')$ is concentrated on the diagonal
\begin{align*}
m \sum_{y \neq y'} \gamma_y^*(y,y') \leq \sum_{y \neq y'} \gamma_y^*(y,y')\ell(y, y') < \delta \Rightarrow \sum_{y \neq y'} \gamma_y^*(y,y') \leq \delta / m
\end{align*}
Since $\risk_p(f^{*}) \leq \alpha$ also holds, summing the two inequalities we get $\risk_p(f^{*}) + \risk_q(f^{*}) \leq 2\alpha + \frac{B+m}{m}\delta$.
\end{proof}

\begin{lemma}
    Suppose $\min_{f \in \mathcal{H}} \risk_{p}(f) < \alpha$, $\max_y W_{1, \ell}(f\# p_{\rm x \mid \rm y}(\cdot \mid y), f\# q_{\rm x \mid \rm y}(\cdot \mid y)) < \beta \in [0, L]$, and $W_{1, \ell}(p_{\rm y}, q_{\rm y}) < \delta$. If $\vert \ell \vert < L$ and the minimum loss for disagreement is given by $M = \min_{y \neq y'} \ell(y, y')$, then $\CDA(\lambda)$ holds with $\lambda = 2 \alpha + 2 \cdot \frac{L}{M} \cdot \delta + \beta \cdot (1 - \TV(p_{\rm y}, q_{\rm y}))$.

    \fix{
    This is better if:
    \begin{align*}
        2\alpha + \frac{L + M}{M} \cdot \delta > 2 \alpha + 2 \cdot \frac{L}{M} \cdot \delta + \beta \cdot (1 - \TV(p_{\rm y}, q_{\rm y})) \\
        \delta > \frac{L}{M} \cdot \delta + \beta \cdot (1 - \TV(p_{\rm y}, q_{\rm y})) \\
        0 > \delta \cdot \left( 1 - \frac{L}{M} \right) >  \beta \cdot (1 - \TV(p_{\rm y}, q_{\rm y})).
    \end{align*}
    Always weaker with same assumptions ... my failed attempt to inject a dependence on the class conditionals.
    Maybe remove.
    }
\end{lemma}
\fix{Alex: TODO move proof to appendix eventually.}
\begin{proof}
    First note that the assumption on $W_{1, \ell}(p_{\rm y}, q_{\rm y}) < \delta$ can be transferred to total variation:
    \begin{equation*}
        M \cdot \TV(p_{\rm y}, q_{\rm y}) \leq
        W_{1, \ell}(p_{\rm y}, q_{\rm y}) \leq L \cdot \TV(p_{\rm y}, q_{\rm y}),
    \end{equation*}
    which holds by switching to the Kronecker cost function.
    Thus, 
    \begin{equation*}
        \TV(p_{\rm y}, q_{\rm y}) \leq
        \frac{1}{M} \cdot \delta.
    \end{equation*}
    Now using Lemma~\ref{lem:transport-partial-decomp}, we have a variant of Corollary~\ref{cor0},
    \begin{align*}
        \risk_{q}(f)
        &\leq \risk_{p}(f) + L \cdot \TV(p_{\rm y}, q_{\rm y}) + \expect_{({y}, {y}') \sim \gamma_{\rm y}^{\TV}}[W_{1, \ell}(f \# p_{\rm x \mid y}(\cdot \mid y), f \# q_{\rm x \mid y}(\cdot \mid {y}'))] \\
        &\leq \alpha + \frac{L}{M} \cdot \delta + \expect_{({y}, {y}') \sim \gamma_{\rm y}^{\TV}}[W_{1, \ell}(f \# p_{\rm x \mid y}(\cdot \mid y), f \# q_{\rm x \mid y}(\cdot \mid {y}'))] \\
        &= \alpha + \frac{L}{M} \cdot \delta + \sum_{y} \gamma_{\rm y}^{\TV}(y, y') \cdot W_{1, \ell}(f \# p_{\rm x \mid y}(\cdot \mid y), f \# q_{\rm x \mid y}(\cdot \mid {y})) \\
        & \quad \quad + \sum_{({y}, {y}') \colon {y} \neq {y}'} \gamma_{\rm y}^{\TV}(y, y') \cdot W_{1, \ell}(f \# p_{\rm x \mid y}(\cdot \mid y), f \# q_{\rm x \mid y}(\cdot \mid {y}')) \\
        &\leq \alpha + 2 \cdot \frac{L}{M} \cdot \delta + \beta \cdot \sum_{\hat{y}} \gamma_{\rm y}^{\TV}(y, y') + L \cdot \sum_{(\hat{y}, \hat{y}') \colon \hat{y} \neq \hat{y}'} \gamma_{\rm y}^{\TV}(y, y').
    \end{align*}
    Notice that we also have,
    \begin{align*}
        \sum_{({y}, {y}') \colon {y} \neq {y}'} \gamma_{f}^{\TV}(y, y') 
        = \sum_{{y}, {y}'} \gamma_{\rm y}^{\TV}(y, y') \cdot \llbracket \hat{y} \neq \hat{y}' \rrbracket
        = \TV(f\#p_{\rm x}, f\#q_{\rm x})
        < \frac{1}{M} \cdot \delta.
    \end{align*}
    Then together we have,
    \begin{align*}
        \risk_{q}(f)
        &\leq \alpha + \frac{L}{M} \cdot \delta + \beta \cdot \sum_{\hat{y}} \gamma_{\rm y}^{\TV}(y, y') + \frac{L}{M} \cdot \delta \\
        &= \alpha + 2 \cdot \frac{L}{M} \cdot \delta + \beta \cdot \sum_{\hat{y}} \gamma_{\rm y}^{\TV}(y, y') \\
        &= \alpha + 2 \cdot \frac{L}{M} \cdot \delta + \beta \cdot \sum_{\hat{y}} \min(p_{\rm y}(y), q_{\rm y}(y)) \\
        &= \alpha + 2 \cdot \frac{L}{M} \cdot \delta + \beta \cdot (1 - \TV(p_{\rm y}, q_{\rm y})) \\
        &\leq \alpha + 2 \cdot \frac{L}{M} \cdot \delta + \beta.
    \end{align*}
    Here we are using the total variation distance optimal coupling and properties of total variation.
    Thus simply adding $\risk_{p}(f)$ yields the result.
\end{proof}
